# Supplementary material for: A First Step Towards Understanding Real-world Attacks on IoT Devices
Source: arXiv:2003.01218 source file (2020-03-02)
Supplement: Supplementary file 1 [file appendix.tex]

\section{Appendix}
\label{sec:appendix}
%\ref{fig:Human_session} \ref{fig:botsession}

\begin{figure}[]
  \includegraphics[width=\linewidth]{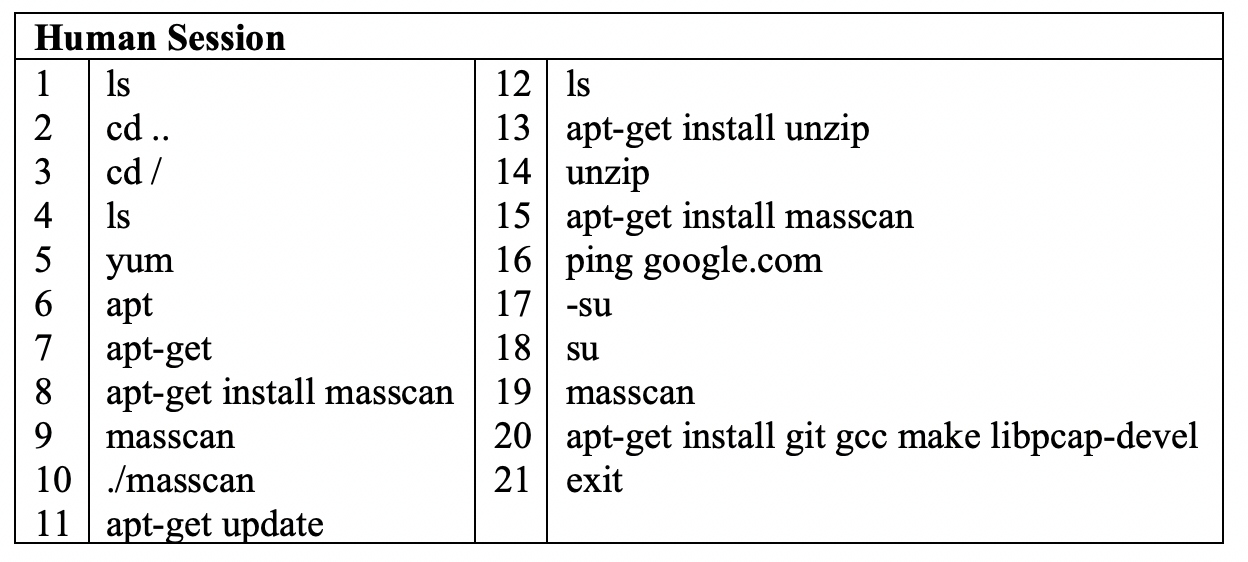}
  \label{fig:Human_session}
\end{figure}
\begin{figure}[]
  \includegraphics[width=\linewidth]{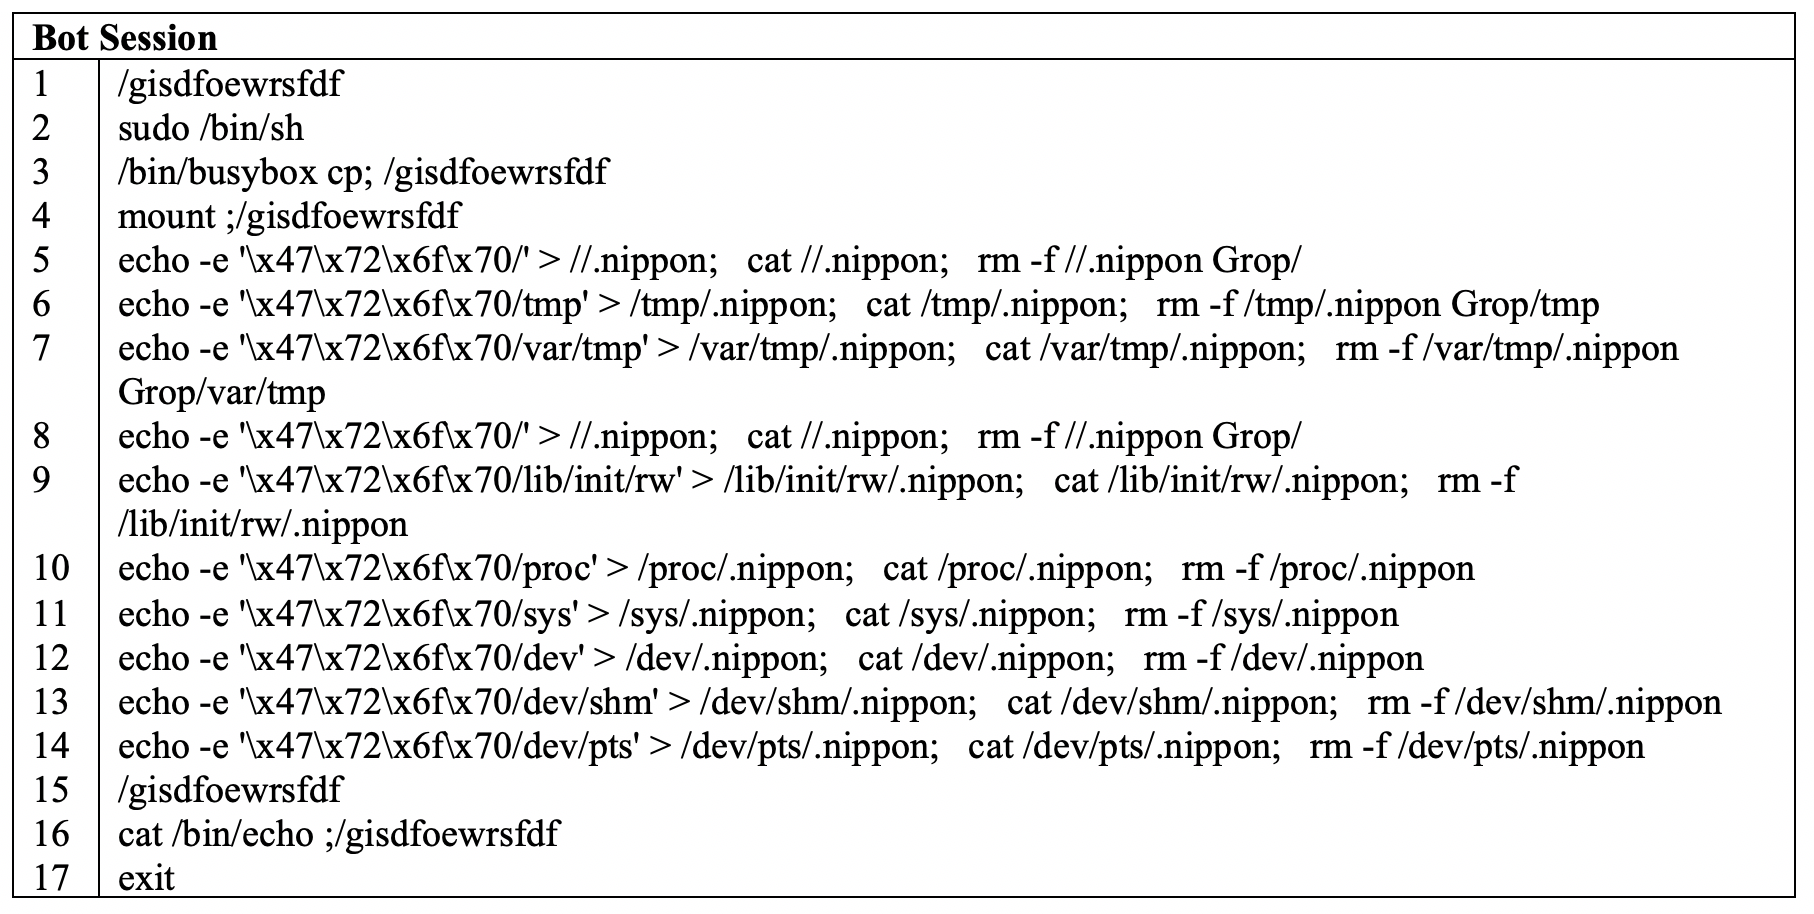}
  \label{fig:botsession}
\end{figure}

%%% Local Variables:
%%% mode: latex
%%% TeX-master: "main"
%%% End:
